# Supplementary material for: MM-CamObj: A Comprehensive Multimodal Dataset for Camouflaged Object Scenarios
Source: arXiv:2409.16084 source file (2024-09-24)
Supplement: Supplementary file 1 [file Appendix.tex]

\begin{figure}[!t]
    \centering
    \includegraphics[width=0.99\linewidth]{AnonymousSubmission/LaTeX/FIGS/figptprompt_appendix.pdf}
    \caption{The detiled Prompt of GPT-4o for constructing our CamObj-Align dataset.}
    \label{fig:gpt4o-align}
\end{figure}

\begin{figure}[!t]
    \centering
    \includegraphics[width=0.99\linewidth]{AnonymousSubmission/LaTeX/FIGS/figsftprompt_appendix.pdf}
    \caption{The detiled Prompt of GPT-4o for constructing our CamObj-Instruct dataset.}
    \label{fig:gpt4o-instruct}
\end{figure}

\section{Detail Prompt of GPT-4o}

% 对于CamObj-Align和CamObj-Instruct，我们使用GPT-4o生成了11,363张伪装图像的相应问答对。图\ref{fig:gpt4o-align}展示了我们在构建CamObj-Align时使用的GPT-4o提示词，而图\ref{fig:gpt4o-instruct}则展示了我们在构建CamObj-Instruct时使用的GPT-4o提示词。
For both CamObj-Align and CamObj-Instruct, we leverage GPT-4o to generate corresponding question-answer pairs for 11,363 camouflage images. Figure \ref{fig:gpt4o-align} illustrates the GPT-4o prompt employed in constructing CamObj-Align, while Figure \ref{fig:gpt4o-instruct} shows the GPT-4o prompt used in developing CamObj-Instruct.

\section{Statistic Information of MM-CamObj and CamObj-Bench}

% 如图\ref{fig:dataset_distribution}和图\ref{fig:bench_distribution}所示，我们首先展示了MM-CamObj数据集中11,363张图像以及CmaObj-Bench数据集中600张图像的整体分布情况。随后，如图\ref{fig:withoutbench_class_distribution_page_1,fig:withoutbench_class_distribution_page_2,fig:bench_class_distribution_page_1,fig:bench_class_distribution_page_2}所示，我们进一步展示了MM-CamObj和CamObj-Bench数据集中不同类别标签的分布情况。
As shown in Figures \ref{fig:dataset_distribution} and \ref{fig:bench_distribution}, we first present the overall distribution of 11,363 images in the MM-CamObj dataset and 600 images in the CmaObj-Bench. Subsequently, as illustrated in Figures \ref{fig:withoutbench_class_distribution_page_1}, \ref{fig:withoutbench_class_distribution_page_2}, \ref{fig:bench_class_distribution_page_1}, and \ref{fig:bench_class_distribution_page_2}, we further demonstrate the distribution of category labels within the MM-CamObj and CamObj-Bench.

\begin{figure*}
    \centering
    \includegraphics[width=0.99\linewidth]{FIGS/WithoutBench_plot.pdf}
    \caption{Data distribution of the MM-CamObj (a) Object Count Distribution: The distribution of object counts per image. (b) Area Ratio Distribution: The distribution of the total area ratio of objects within images. (c) Dataset Source Distribution: The distribution of dataset sources. The  plots provides a comprehensive overview of key characteristics within the bench dataset.}
    \label{fig:dataset_distribution}
\end{figure*}

\begin{figure*}
    \centering
    \includegraphics[width=0.99\linewidth]{FIGS/Bench_plot.pdf}
    \caption{Data distribution of the CamObj-Bench (a) Object Count Distribution: The distribution of object counts per image. (b) Area Ratio Distribution: The distribution of the total area ratio of objects within images. {(c) Dataset Source Distribution: }The distribution of dataset sources. The  plots provides a comprehensive overview of key characteristics within the bench dataset.}
    \label{fig:bench_distribution}
\end{figure*}

\begin{figure*}
    \centering
    \includegraphics[width=0.99\linewidth]{FIGS/WithoutBench_class_distribution_page_1.pdf}
    \caption{Class distribution for the MM-CamObj (Page 1).}
    \label{fig:withoutbench_class_distribution_page_1}
\end{figure*}

\begin{figure*}
    \centering
    \includegraphics[width=0.99\linewidth]{FIGS/WithoutBench_class_distribution_page_2.pdf}
    \caption{Class distribution for the MM-CamObj (Page 2).}
    \label{fig:withoutbench_class_distribution_page_2}
\end{figure*}

\begin{figure*}
    \centering
    \includegraphics[width=0.99\linewidth]{FIGS/Bench_class_distribution_page_1.pdf}
    \caption{Class distribution for the CamObj-Bench (Page 1).}
    \label{fig:bench_class_distribution_page_1}
\end{figure*}

\begin{figure*}
    \centering
    \includegraphics[width=0.99\linewidth]{FIGS/Bench_class_distribution_page_2.pdf}
    \caption{Class distribution for the CamObj-Bench (Page 2).}
    \label{fig:bench_class_distribution_page_2}
\end{figure*}

% benchmark的更多示例（画图, 可以画大点, 每一个任务放3个示例）【ywz】
\section{More Visualization on Data Samples of CamObj-Bench}

% 我们进一步展示了各任务的更多可视化样本，包括Easy VQA（图 \ref{fig:easyVQAsample}）、Hard VQA（图 \ref{fig:hardVQAsample}）、Bbox定位（图 \ref{fig:BboxSample}）、数量选择（图 \ref{fig:countSample}）、图像描述（图 \ref{fig:imagecaptionSample1} 和 \ref{fig:imagecaptionSample2}）、Mask匹配（图 \ref{fig:maskmatchSample}）以及Mask TF任务（图 \ref{fig:maskTFSample}）。
We further present additional visual samples for various tasks, including Easy VQA (Figure \ref{fig:easyVQAsample}), Hard VQA (Figure \ref{fig:hardVQAsample}), Bbox Location (Figure \ref{fig:BboxSample}), Count Choice (Figure \ref{fig:countSample}), Image Caption (Figures \ref{fig:imagecaptionSample1} and \ref{fig:imagecaptionSample2}), Mask Match (Figure \ref{fig:maskmatchSample}), and Mask TF (Figure \ref{fig:maskTFSample}) tasks.

\begin{figure*}[htbp]
    \centering
    \includegraphics[width=0.99\linewidth]{FIGS/easyVQAsample.pdf}
    \caption{Some samples of Easy VQA question in CamObj-Bench.}
    \label{fig:easyVQAsample}
\end{figure*}

\begin{figure*}[htbp]
    \centering
    \includegraphics[width=0.99\linewidth]{FIGS/hardVQAsample.pdf}
    \caption{Some samples of Hard VQA question in CamObj-Bench.}
    \label{fig:hardVQAsample}
\end{figure*}

\begin{figure*}[htbp]
    \centering
    \includegraphics[width=0.99\linewidth]{FIGS/BboxSample.pdf}
    \caption{Some samples of Bbox location question in CamObj-Bench.}
    \label{fig:BboxSample}
\end{figure*}

\begin{figure*}[htbp]
    \centering
    \includegraphics[width=0.99\linewidth]{FIGS/countSample.pdf}
    \caption{Some samples of Count choice question in CamObj-Bench.}
    \label{fig:countSample}
\end{figure*}

\begin{figure*}[htbp]
    \centering
    \includegraphics[width=0.99\linewidth]{FIGS/imagecaptionSample1.pdf}
    \caption{Some samples of Image caption question (Sample 1) in CamObj-Bench.}
    \label{fig:imagecaptionSample1}
\end{figure*}

\begin{figure*}[htbp]
    \centering
    \includegraphics[width=0.99\linewidth]{FIGS/imagecaptionSample2.pdf}
    \caption{Some samples of Image caption question (Sample 2) in CamObj-Bench.}
    \label{fig:imagecaptionSample2}
\end{figure*}

\begin{figure*}[htbp]
    \centering
    \includegraphics[width=0.99\linewidth]{FIGS/maskmatchSample.pdf}
    \caption{Some samples of Mask Match question in CamObj-Bench.}
    \label{fig:maskmatchSample}
\end{figure*}

\begin{figure*}[htbp]
    \centering
    \includegraphics[width=0.99\linewidth]{FIGS/maskTFSample.pdf}
    \caption{Some samples of Mask TF question in CamObj-Bench.}
    \label{fig:maskTFSample}
\end{figure*}

% 模型的回答结果（将问题以及模型的回答, 画图, 每个任务放两个示例, 包含Llava-7B/CamObj-Llava-7B以及GPT-4o）【ywz】

% 2 Mask: 4,  GPT-4o,  3 对 1 错；Llava/Camo 4 错

% E VQA：L 1 对 1错； C 2 对；GPT-4o 2 对
% H VQA 1对1错
% Bbox C 接近 GT
% Image Caption 读 3物体 标记
% Count  L 1 对 1错； C 2 对；GPT-4o 1 对 1错

\section{Case Studies}

% 为了更加清晰地展示MM-CamObj和CamObj-Llava的优势，我们进行了详尽的案例分析。在CamObj-Bench的七项任务中，我们对GPT-4o、Llava-v1.5-7B \cite{llava1_5} 以及我们的CamObj-Llava-7B的回答结果进行了全面的可视化。具体而言，如图\ref{fig:imagecaption1}、\ref{fig:imagecaption2}、\ref{fig:imagecaption3}、\ref{fig:imagecaption4} 和 \ref{fig:imagecaption5} 所示，我们展示了三种模型在图像描述任务中的表现。图\ref{fig:easyVQA1} 和 \ref{fig:easyVQA2} 展示了在简单VQA任务中的可视化结果。图\ref{fig:hardVQA1} 和 \ref{fig:hardVQA2} 展示了在复杂VQA任务中的表现。图\ref{fig:bbox1} 和 \ref{fig:bbox2} 展示了在边界框定位任务中的结果。图\ref{fig:count1} 和 \ref{fig:count2} 展示了在计数选择任务中的表现。图\ref{fig:maskmatch1} 和 \ref{fig:maskmatch2} 展示了在遮罩匹配任务中的可视化结果。最后，图\ref{fig:maskTF1} 和 \ref{fig:maskTF2} 展示了遮罩真伪任务中的表现。
To clearly demonstrate the advantages of MM-CamObj and CamObj-Llava, we conducted detailed case studies. In the seven tasks of CamObj-Bench, we comprehensively visualized the responses of GPT-4o, Llava-v1.5-7B \cite{llava1_5}, and our CamObj-Llava-7B. Specifically, as shown in Figures \ref{fig:imagecaption1}, \ref{fig:imagecaption2}, \ref{fig:imagecaption3}, \ref{fig:imagecaption4}, and \ref{fig:imagecaption5}, we present the performance of the three models on the Image Caption task. Figures \ref{fig:easyVQA1} and \ref{fig:easyVQA2} illustrate the visual results on the Easy VQA task. Figures \ref{fig:hardVQA1} and \ref{fig:hardVQA2} depict the performance on the Hard VQA task. Figures \ref{fig:bbox1} and \ref{fig:bbox2} show the results on the Bbox Location task. Figures \ref{fig:count1} and \ref{fig:count2} present the performance on the Count Choice task. Figures \ref{fig:maskmatch1} and \ref{fig:maskmatch2} illustrate the visual results on the Mask Match task. Finally, Figures \ref{fig:maskTF1} and \ref{fig:maskTF2} show the performance on the Mask TF task.

%Image Caption
\begin{figure*}
    \centering
    \includegraphics[width=0.905\linewidth]{FIGS/imagecaption1.pdf}
    \caption{A sample case of Image Caption question,  and answer from GPT-4o, Llava-v1.5-7B, CamObj-Llava-7B. {Green} highlights the right answer. {Red} highlights the wrong answer.}
    \label{fig:imagecaption1}
\end{figure*}

\begin{figure*}
    \centering
    \includegraphics[width=0.905\linewidth]{FIGS/imagecaption2.pdf}
    \caption{A sample case of Image Caption question,  and answer from GPT-4o, Llava-v1.5-7B, CamObj-Llava-7B. {Green} highlights the right answer. {Red} highlights the wrong answer.}
    \label{fig:imagecaption2}
\end{figure*}

\begin{figure*}
    \centering
    \includegraphics[width=0.905\linewidth]{FIGS/imagecaption3.pdf}
    \caption{A sample case of Image Caption question,  and answer from GPT-4o, Llava-v1.5-7B, CamObj-Llava-7B. {Green} highlights the right answer. {Red} highlights the wrong answer.}
    \label{fig:imagecaption3}
\end{figure*}

\begin{figure*}
    \centering
    \includegraphics[width=0.905\linewidth]{FIGS/imagecaption4.pdf}
    \caption{A sample case of Image Caption question,  and answer from GPT-4o, Llava-v1.5-7B, CamObj-Llava-7B. {Green} highlights the right answer. {Red} highlights the wrong answer.}
    \label{fig:imagecaption4}
\end{figure*}

\begin{figure*}
    \centering
    \includegraphics[width=0.905\linewidth]{FIGS/imagecaption5.pdf}
    \caption{A sample case of Image Caption question,  and answer from GPT-4o, Llava-v1.5-7B, CamObj-Llava-7B. {Green} highlights the right answer. {Red} highlights the wrong answer.}
    \label{fig:imagecaption5}
\end{figure*}

% easyVQA1
\begin{figure*}
    \centering
    \includegraphics[width=0.905\linewidth]{FIGS/easyVQA1.pdf}
    \caption{A sample case of Easy VQA question,  and answer from GPT-4o, Llava-v1.5-7B, CamObj-Llava-7B.}
    \label{fig:easyVQA1}
\end{figure*}

% easyVQA2
\begin{figure*}
    \centering
    \includegraphics[width=0.905\linewidth]{FIGS/easyVQA2.pdf}
    \caption{A sample case of Easy VQA question,  and answer from GPT-4o, Llava-v1.5-7B, CamObj-Llava-7B.}
    \label{fig:easyVQA2}
\end{figure*}

% hardVQA1
\begin{figure*}
    \centering
    \includegraphics[width=0.905\linewidth]{FIGS/hardVQA1.pdf}
    \caption{A sample case of Hard VQA question,  and answer from GPT-4o, Llava-v1.5-7B, CamObj-Llava-7B.}
    \label{fig:hardVQA1}
\end{figure*}

% hardVQA2
\begin{figure*}
    \centering
    \includegraphics[width=0.905\linewidth]{FIGS/hardVQA2.pdf}
    \caption{A sample case of Hard VQA question,  and answer from GPT-4o, Llava-v1.5-7B, CamObj-Llava-7B.}
    \label{fig:hardVQA2}
\end{figure*}

% 第一张图 - bbox1
\begin{figure*}
    \centering
    \includegraphics[width=0.905\linewidth]{FIGS/bbox1.pdf}
    \caption{A sample case of Bbox Location question,  and answer from GPT-4o, Llava-v1.5-7B, CamObj-Llava-7B.}
    \label{fig:bbox1}
\end{figure*}

% 第二张图 - bbox2
\begin{figure*}
    \centering
    \includegraphics[width=0.905\linewidth]{FIGS/bbox2.pdf}
    \caption{A sample case of Bbox Location question,  and answer from GPT-4o, Llava-v1.5-7B, CamObj-Llava-7B.}
    \label{fig:bbox2}
\end{figure*}

% 第三张图 - count1
\begin{figure*}
    \centering
    \includegraphics[width=0.905\linewidth]{FIGS/count1.pdf}
    \caption{A sample case of Count choice question,  and answer from GPT-4o, Llava-v1.5-7B, CamObj-Llava-7B.}
    \label{fig:count1}
\end{figure*}

% 第四张图 - count2
\begin{figure*}
    \centering
    \includegraphics[width=0.905\linewidth]{FIGS/count2.pdf}
    \caption{A sample case of Count choice question,  and answer from GPT-4o, Llava-v1.5-7B, CamObj-Llava-7B.}
    \label{fig:count2}
\end{figure*}

% 第十一张图 - maskmatch1
\begin{figure*}
    \centering
    \includegraphics[width=0.905\linewidth]{FIGS/maskmatch1.pdf}
    \caption{A sample case of Mask Match question,  and answer from GPT-4o, Llava-v1.5-7B, CamObj-Llava-7B.}
    \label{fig:maskmatch1}
\end{figure*}

% 第十二张图 - maskmatch2
\begin{figure*}
    \centering
    \includegraphics[width=0.905\linewidth]{FIGS/maskmatch2.pdf}
    \caption{A sample case of Mask Match question,  and answer from GPT-4o, Llava-v1.5-7B, CamObj-Llava-7B.}
    \label{fig:maskmatch2}
\end{figure*}

% 第九张图 - maskTF1
\begin{figure*}
    \centering
    \includegraphics[width=0.905\linewidth]{FIGS/maskTF1.pdf}
    \caption{A sample case of Mask TF question,  and answer from GPT-4o, Llava-v1.5-7B, CamObj-Llava-7B.}
    \label{fig:maskTF1}
\end{figure*}

% 第十张图 - maskTF2
\begin{figure*}
    \centering
    \includegraphics[width=0.905\linewidth]{FIGS/maskTF2.pdf}
    \caption{A sample case of Mask TF question,  and answer from GPT-4o, Llava-v1.5-7B, CamObj-Llava-7B.}
    \label{fig:maskTF2}
\end{figure*}
